# Supplementary material for: Cluster Glasses of Semiflexible Ring Polymers
Source: arXiv:1309.1061 source file (2013-12-11)
Supplement: Supplementary file 1 [file SuppMat_LJ13656_v2.pdf]

# SUPPLEMENTAL MATERIAL

# Cluster Glasses of Semiflexible Ring Polymers

Mohammed Zakaria Slimani,[1] Petra Bacova,[2,3] Marco Bernabei,[1,4]
Arturo Narros,[5] Christos N. Likos,[5] and Angel J. Moreno[1,3,6,*]

[1]*Donostia International Physics Center,*
*Paseo Manuel de Lardizabal 4, E-20018 San Sebastián, Spain.*
[2]*Departamento de Física de Materiales,*
*Universidad del País Vasco (UPV/EHU),*
*Apartado 1072, E-20080 San Sebastián, Spain.*
[3]*Materials Physics Center MPC, Paseo Manuel*
*de Lardizabal 5, E-20018 San Sebastián, Spain.*
[4]*Departament de Fisica Fonamental, Universitat de Barcelona,*
*Martí i Franquès 1, E-08028 Barcelona, Spain.*
[5]*Faculty of Physics, University of Vienna,*
*Boltzmanngasse 5, A-1090 Vienna, Austria.*
[6]*Centro de Física de Materiales (CSIC, UPV/EHU),*
*Paseo Manuel de Lardizabal 5, E-20018 San Sebastián, Spain.*

[*]Corresponding author: wabmosea@ehu.es

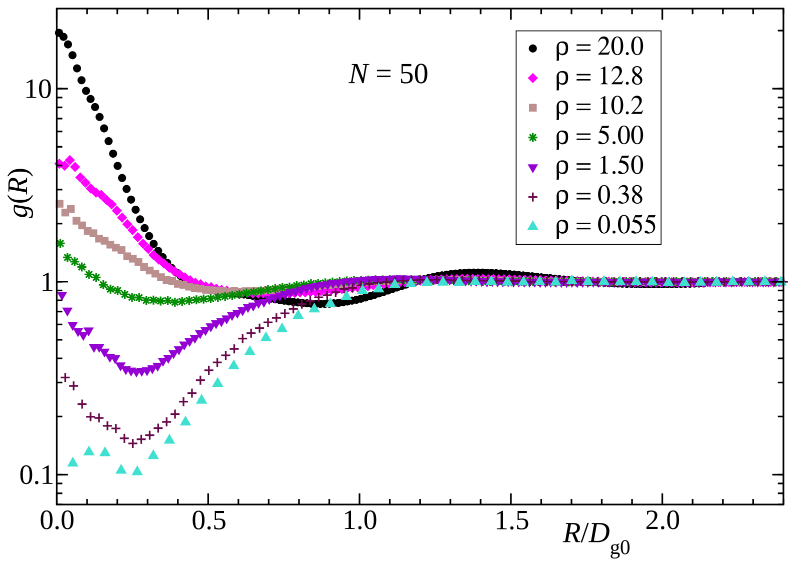


Fig. S1: For $N = 50$, radial distribution function of the centers-of-mass at different densities (see legend).

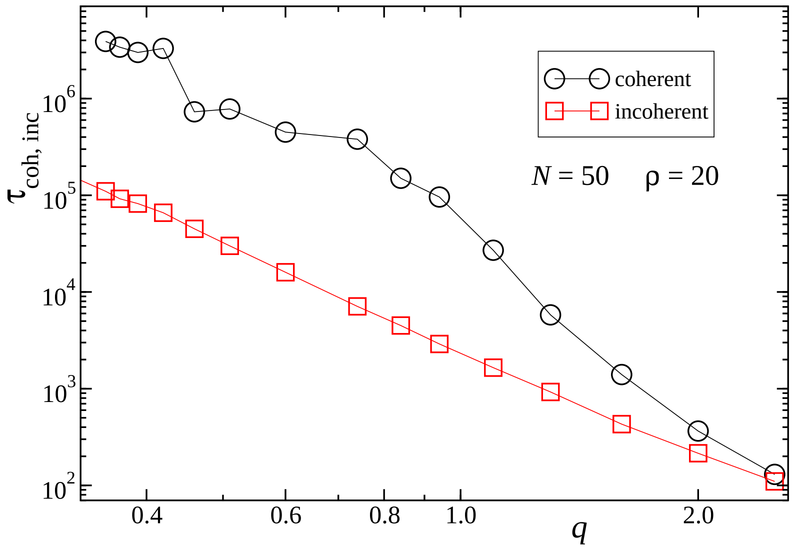


Fig. S2: For $N = 50$ and $\rho = 20$, $q$-dependence of the relaxation times of the scattering functions of the centers-of-mass. Circles and squares are data for the coherent and incoherent functions, respectively.

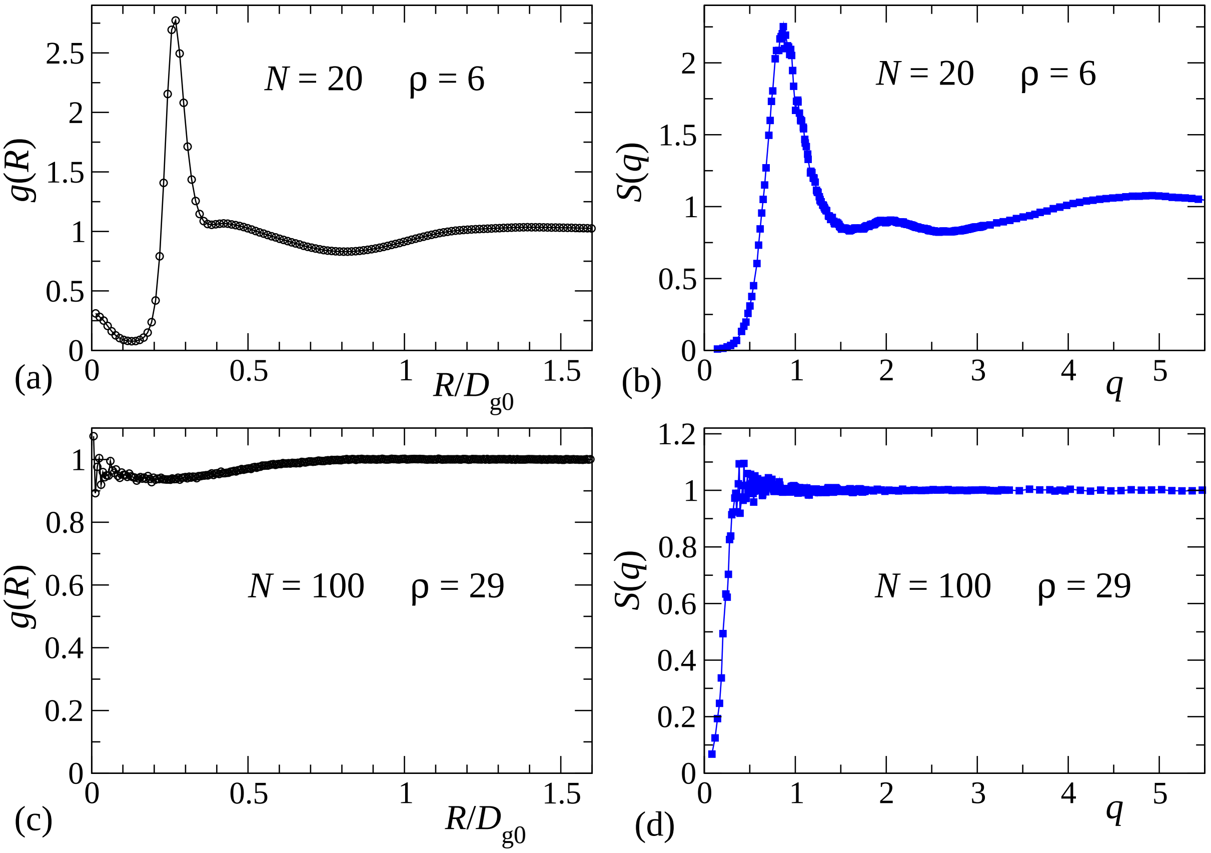


Fig. S3: Radial distributions functions [(a) and (c)] and static structure factors [(b) and (d)] for the centers-of-mass of non-clustering semiflexible rings. (a) and (b): rings of $N = 20$ at $\rho = 6$, which corresponds to a monomer density $\rho_{\rm m} = 0.59$. (c) and (d): rings of $N = 100$ at $\rho = 29$, which corresponds to a monomer density $\rho_{\rm m} = 0.28$.

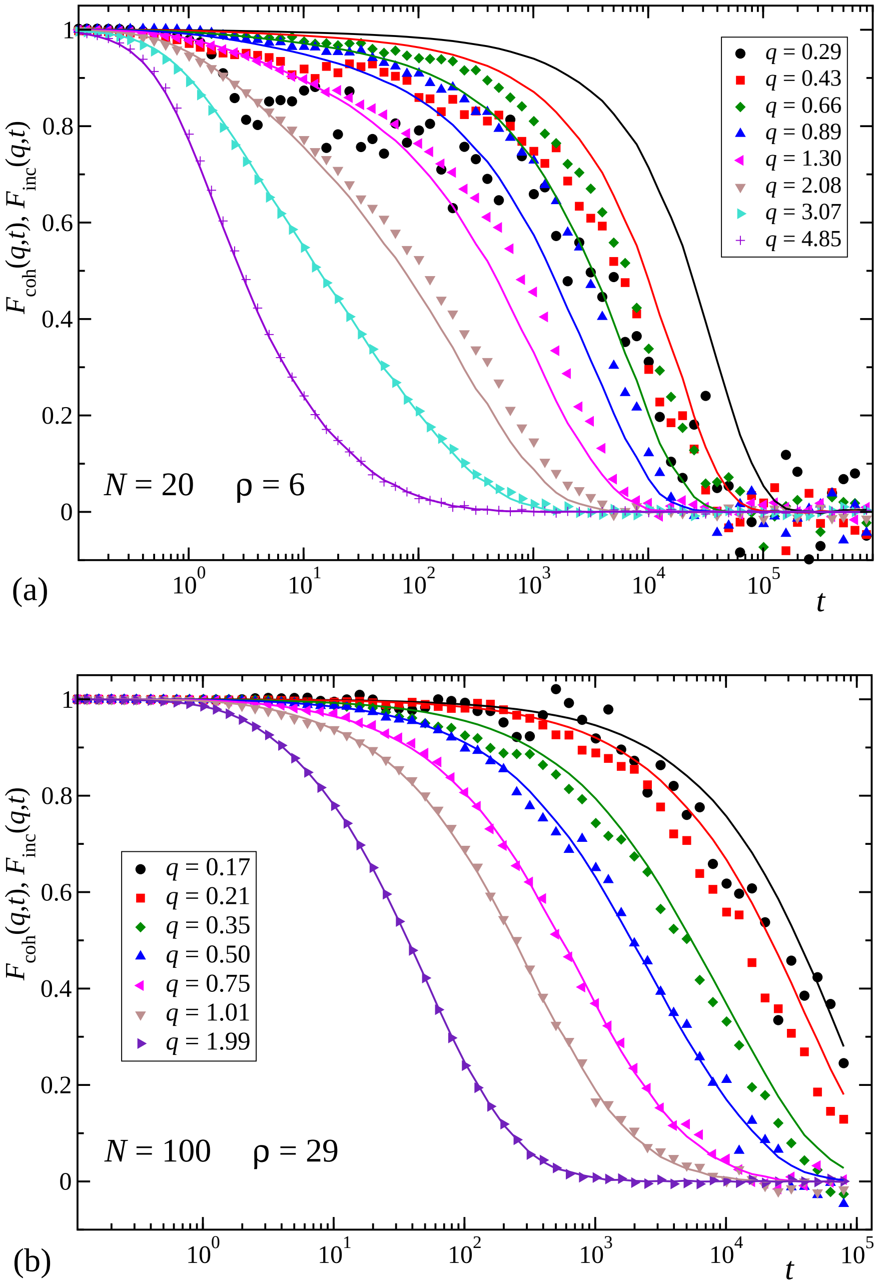


Fig. S4: Coherent (symbols) and incoherent (lines) scattering functions of the centers-of-mass at different $q$-values. (a): Data for rings of $N = 20$ at $\rho = 6$; (b): Data for rings of $N = 100$ at $\rho = 29$.

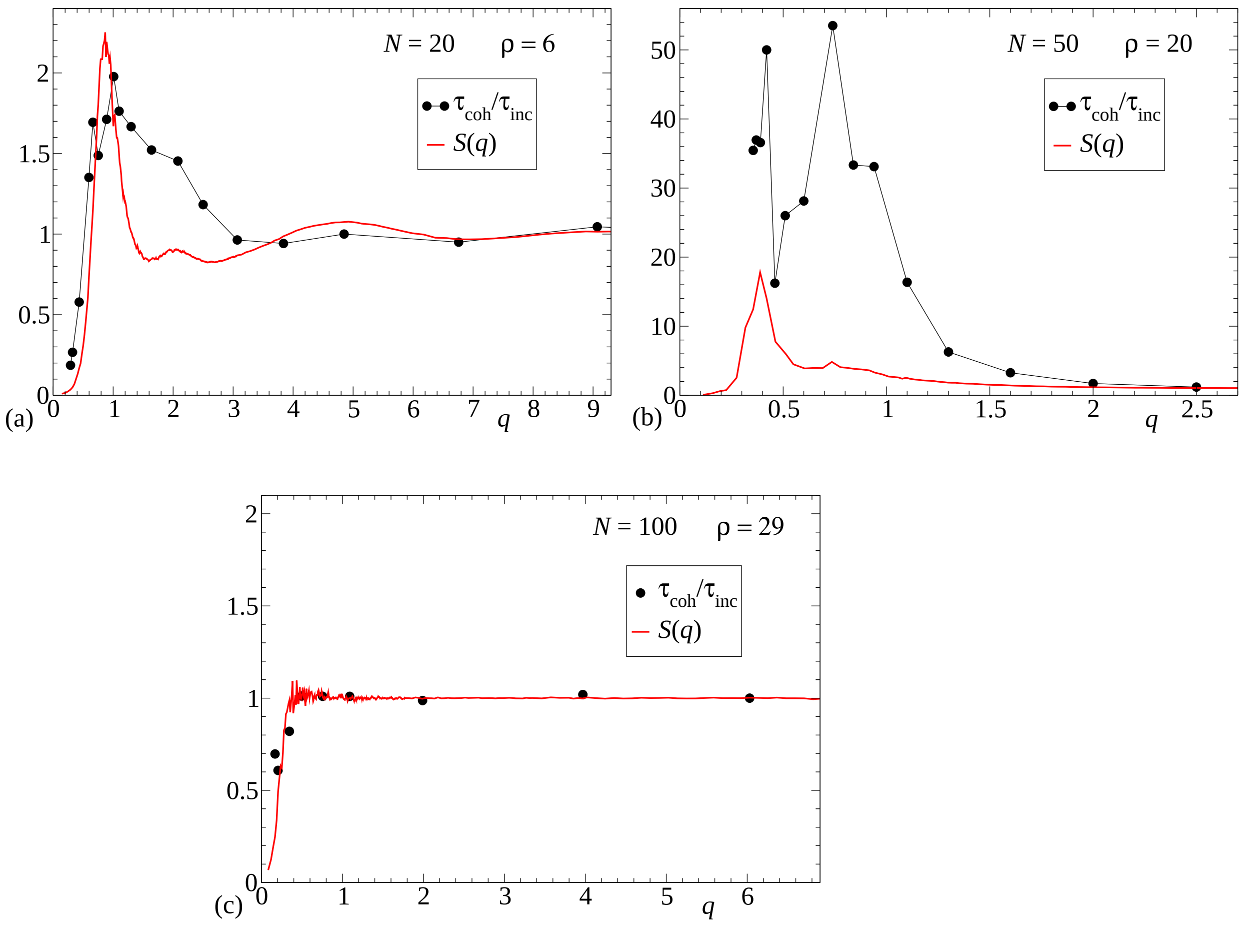


Fig. S5: Full black circles: $q$-dependence of the ratio of the coherent to the incoherent relaxation time. Thick red lines: static structure factor of the centers-of-mass. Data in different panels correspond, for each polymerization degree $N$, to the highest investigated ring density $\rho$. The values of these quantities and of the monomer density $\rho_{\rm m}$ are (a): $N = 20$, $\rho = 6$, $\rho_{\rm m} = 0.59$; (b): $N = 50$, $\rho = 20$, $\rho_{\rm m} = 0.45$; (c) $N = 100$, $\rho = 29$, $\rho_{\rm m} = 0.28$.

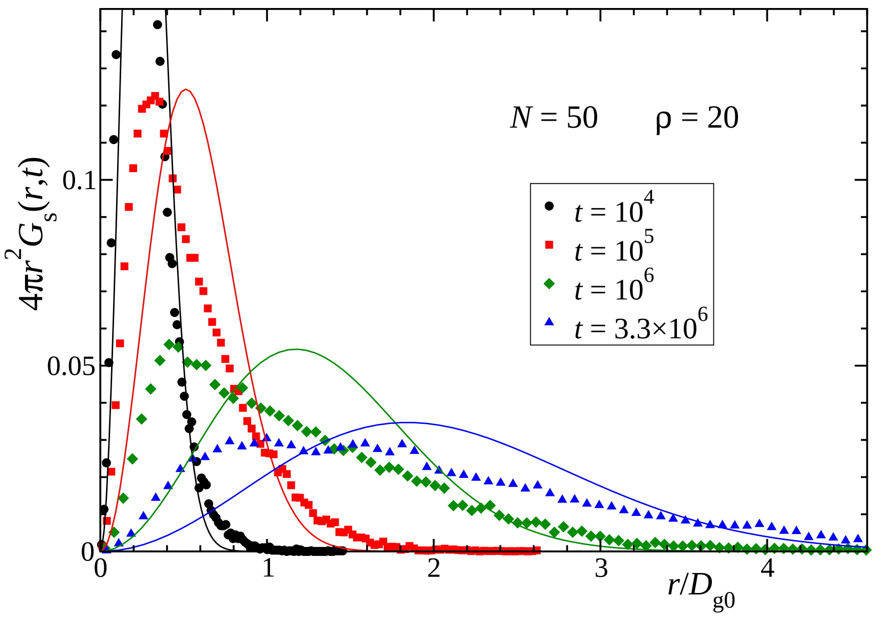


Fig. S6: Van Hove self-correlation function of the centers-of-mass, for $N = 50$, $\rho = 20$ and at different selected times. The functions are multiplied by the phase factor $4\pi r^2$ in order to represent the normalized distribution of displacements. Symbols are simulation data. Lines are calculated by using Gaussian functions, $G_s(r,t) = (3/2\pi\langle r^2(t)\rangle)^{3/2}\exp[-3r^2/2\langle r^2(t)\rangle]$, with $\langle r^2(t)\rangle$ the mean squared displacement obtained from the simulation.

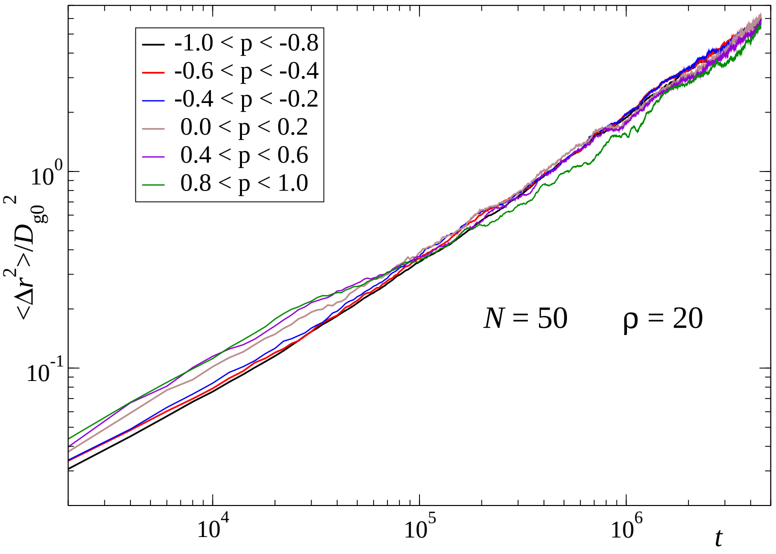


Fig. S7: For $N = 50$ and $\rho = 20$, mean squared displacement, normalized by $D_{g0}^2$, of the centers-of-mass of the rings, according to their prolateness $p$ at $t = 0$. The intervals of $p$ are given in the legend.
